# Supplementary material for: How Does the Task Landscape Affect MAML Performance?
Source: arXiv:2010.14672 source file (2022-08-09)
Supplement: Supplementary file 1 [file Appendix_experiments.tex]

\section{Additional Experimental Details and Results}

\subsection{Further Experimental Details}

\subsubsection{Omniglot Experiment}

\subsection{Linear Regression}

\subsection{Logistic Regression}

\subsection{Linear Regression with Representation Learning}
