# Supplementary material for: How Does the Task Landscape Affect MAML Performance?
Source: arXiv:2010.14672 source file (2022-08-09)
Supplement: Supplementary file 3 [file Appendix_Nonlinear.tex]

%!TEX root = main.tex

\begin{comment}
\section{Nonlinear Analysis}
\subsection{General Strongly Convex and Smooth Functions}

\begin{proposition} \label{prop:sc}
Suppose there are two tasks with smooth and strongly convex loss functions $f_1$ and $f_2$. The smoothness and strong convexity parameters for task 1 are $L_1$ and $\mu_1$, and the smoothness and strong convexity parameters for task 2 are $L_2$ and $\mu_2$, respectively.
Suppose task 1 is the hard task and task 2 is the easy task, i.e. $\mu_2 > \mu_1$, and further suppose that $L_2 > L_1$. Also let the step size $\alpha = 1/L_2$.
Let $\mathbf{w}_{1,\ast}$ and $\mathbf{w}_{2,\ast}$ be the optimal solutions for the first and second tasks, respectively, and let $\mathbf{w}_{MAML}$ be the optimal solution for MAML. Then the following holds:
\begin{align}
    \|\mathbf{w}_{MAML} - \mathbf{w}_{1,\ast}\|_2 \leq \frac{(L_2 - \mu_2)^2}{(L_2 - L_1)\mu_1 \beta_1}\|\mathbf{w}_{MAML} - \mathbf{w}_{2,\ast}\|_2
\end{align}
where $\beta_1 = \left(\frac{\sqrt{L_1/\mu_1} - 1}{\sqrt{L_1/\mu_1} + 1} \right)^2$, i.e. $\mathbf{w}_{MAML}$ is closer to the solution for the hard task as long as $\frac{(L_2 - \mu_2)^2}{(L_2 - L_1)\mu_1 \beta_1} < 1$. 
% {\color{red} However, this only holds in very specific settings: we need (roughly) $\mu_2 < L_1$ and $L_2 < \mu_1 + \mu_2$. In simulations, if a task has large data variance, it may still have large condition number, i.e. $L_2 \gg \mu_2$, which makes it unlikely that $L_2 < \mu_1 + \mu_2$ since $\mu_1$ is small as task 1 is hard.}
\end{proposition}
\begin{proof}

\end{proof}

\end{comment}

\section{Proof of Theorem \ref{lem:sc}}

In this section we prove Theorem \ref{lem:sc}.  We first show a general result.

\begin{lemma}\label{prop:hess}

Let $\mathbf{w}_{MAML} \in \mathbb{R}^D$ be a stationary point of the MAML objective \ref{exp_test} with $m=\infty$ whose Hessians of the task loss functions are bounded and positive definite, i.e. $\mathbf{w}_{MAML}$ satisfies 
\begin{align}
    \beta_1 \mathbf{I}_{D} \preceq \nabla^2 f_1 (\mathbf{w}_{MAML}) \preceq L_1 \mathbf{I}_{D}, \quad \beta_2 \mathbf{I}_{D} \preceq \nabla^2 f_2 (\mathbf{w}_{MAML}) \preceq L_2 \mathbf{I}_{D}
\end{align}
for some $L_1 \geq \beta_1 > 0$ and $L_2 \geq \beta_2 > 0$. Suppose that $\beta_2 > \beta_1$.
Define $\mathbf{w}_1 \coloneqq \mathbf{w}_{MAML} -\alpha \nabla f_1(\mathbf{w}_{MAML})$ and $\mathbf{w}_2 \coloneqq \mathbf{w}_{MAML} -\alpha \nabla f_2(\mathbf{w}_{MAML})$.
% Suppose that $f_1$ and $f_2$ are strongly convex with parameters $\beta_1$ and $\beta_2$ and smooth with parameters $L_1$ and $L_2$, respectively. Suppose task 2 is the easy task, thus $\beta_2 > \beta_1$ and $L_2 > L_1$, and let $0 < \alpha \leq 1/L_2$.
 Then the following holds for any $\alpha < 1/\max(L_1,L_2)$:
\begin{align}
    \|\nabla f_1(\mathbf{w}_{1})\|_2 \lesssim \frac{1 - \alpha\beta_2}{1 - \alpha L_1} \|\nabla f_2(\mathbf{w}_2)\| + O(\alpha^2).
\end{align}
% Thus, if $\mu_2 > L_1$, then $\|\nabla f_1(\mathbf{w}_{1})\|_2 < \|\nabla f_2(\mathbf{w}_2)\|_2$, assuming O(\alpha^2)..
\end{lemma}

\begin{proof} 
% Recall that the MAML objective is 
% $$ F_{MAML}(\mathbf{w}_{MAML}) \coloneqq \frac{1}{2} f_1(\mathbf{w}_1) + f_2(\mathbf{w}_2)$$, which 

For some vector $\mathbf{w}_{MAML} \in \mathbb{R}^D$, let $\mathbf{H}_1(\mathbf{w}_{MAML}) \coloneqq \nabla^2 f_1(\mathbf{w}_{MAML})$ and $\mathbf{H}_2(\mathbf{w}_{MAML}) = \nabla^2 f_2(\mathbf{w}_{MAML})$ and $\mathbf{g}_1(\mathbf{w}_{MAML}) = \nabla f_1(\mathbf{w}_{1})$ and $\mathbf{g}_2(\mathbf{w}_{MAML}) = \nabla f_2(\mathbf{w}_{2})$, recalling that $\mathbf{w}_1 = \mathbf{w}_{MAML} - \alpha \nabla f_1(\mathbf{w}_{MAML})$ and $\mathbf{w}_2 = \mathbf{w}_{MAML} - \alpha \nabla f_2(\mathbf{w}_{MAML})$.

Recall that the MAML objective in this case is given by 
\begin{align}
    F_\infty(\mathbf{w}) = \frac{1}{2}f_1(\mathbf{w} - \alpha \nabla f_1(\mathbf{w})) + \frac{1}{2}f_2(\mathbf{w} - \alpha \nabla f_2(\mathbf{w})).
\end{align}
After setting the gradient of $F_{\infty}(.)$ equal to zero at $\mathbf{w}_{MAML}$, we find that any stationary point $\mathbf{w}_{MAML}$ of the MAML objective must satisfy
\begin{align}
    (\mathbf{I}_D - \alpha \mathbf{H}_1(\mathbf{w}_{MAML}))\mathbf{g}_1(\mathbf{w}_1) = - (\mathbf{I}_D - \alpha \mathbf{H}_2(\mathbf{w}_{MAML}))\mathbf{g}_2(\mathbf{w}_{2})
\end{align}
Since $\mathbf{H}_2(\mathbf{w}_{MAML})\preceq L_2\mathbf{I}_d$ and $\alpha \leq 1/\max(L_1,L_2)$, $\mathbf{I}_d - \alpha \mathbf{H}_2(\mathbf{w}_{MAML})$ is positive definite with minimum eigenvalue at least $1-\alpha L_2 > 0$. Thus we have 
\begin{align}
    (\mathbf{I}_D - \alpha \mathbf{H}_2(\mathbf{w}_{MAML}))^{-1}(\mathbf{I}_D - \alpha \mathbf{H}_1(\mathbf{w}_{MAML}))\mathbf{g}_1(\mathbf{w}_{1}) = - \mathbf{g}_2(\mathbf{w}_{2})
\end{align}
Taking the norm of both sides and using the fact that $\|\mathbf{A}\mathbf{v}\|_2 \geq \sigma_{\min}(\mathbf{A}) \|\mathbf{v}\|_2$ for any matrix $\mathbf{A}$ and vector $\mathbf{v}$, along with the facts that $\beta_1 \mathbf{I}_D \preceq \mathbf{H}_1(\mathbf{w}_{MAML}) \preceq L_1 \mathbf{I}_D$ and $\beta_2 \mathbf{I}_D \preceq \mathbf{H}_2(\mathbf{w}_{MAML}) \preceq L_2 \mathbf{I}_D$ by assumption, yields
\begin{align}
     \| \mathbf{g}_2(\mathbf{w}_{2})\|_2 &= \|(\mathbf{I}_D - \alpha \mathbf{H}_2(\mathbf{w}_{MAML}))^{-1}(\mathbf{I}_D - \alpha \mathbf{H}_1(\mathbf{w}_{MAML}))\mathbf{g}_1(\mathbf{w}_{1}) \|_2 \nonumber \\
     &\geq \sigma_{\max}^{-1}(\mathbf{I}_D - \alpha \mathbf{H}_2(\mathbf{w}_{MAML})) \sigma_{\min}(\mathbf{I}_D - \alpha \mathbf{H}_1(\mathbf{w}_{MAML})) \|\mathbf{g}_1(\mathbf{w}_{1})\|_2 \nonumber \\
     &\geq  \frac{{1- \alpha {L_1}}}{1 - \alpha {\beta_2}} \|\mathbf{g}_1(\mathbf{w}_{1})\|_2 %\nonumber \\
    %  &= \frac{L_2 - L_1}{L_2 - {\beta_2}} \|\mathbf{g}_1(\mathbf{w}_{1})\|_2 
\end{align}
Next, note that using Taylor expansion, 
\begin{align}
    \mathbf{g}_1(\mathbf{w}_1)  &= \nabla {f}_1(\mathbf{w}_{MAML}) - \alpha \nabla^2 {f}_1(\mathbf{w}_{MAML}) \nabla {f}_1(\mathbf{w}_{MAML}) + O(\alpha^2) \nonumber \\
    &= (\mathbf{I}_D - \alpha \mathbf{H}_1(\mathbf{w}_{MAML}))\mathbf{g}_1 (\mathbf{w}_{MAML})  \\
    \mathbf{g}_2(\mathbf{w}_2)  &= \nabla {f}_2(\mathbf{w}_{MAML}) - \alpha \nabla^2 {f}_2(\mathbf{w}_{MAML}) \nabla {f}_2(\mathbf{w}_{MAML}) + O(\alpha^2) \nonumber \\
    &= (\mathbf{I}_D - \alpha \mathbf{H}_2(\mathbf{w}_{MAML})) \mathbf{g}_2 (\mathbf{w}_{MAML})  
\end{align}
Therefore 
\begin{align}
    \| \mathbf{g}_2(\mathbf{w}_{MAML}&)\|_2 + O(\alpha^2) \nonumber \\
    &\gtrsim \sigma_{\max}^{-1}(\mathbf{I}_D - \alpha \mathbf{H}_2(\mathbf{w}_{MAML})) \sigma_{\min}(\mathbf{I}_D - \alpha \mathbf{H}_1(\mathbf{w}_{MAML})) \frac{1 - \alpha L_1}{1 - \alpha {\beta_2}} \|\mathbf{g}_1(\mathbf{w}_{1})\|_2  \nonumber \\
    &\gtrsim \left(\frac{1 - \alpha L_1}{1 - \alpha {\beta_2}}\right)^2 \|\mathbf{g}_1(\mathbf{w}_{MAML})\|_2, 
\end{align}
i.e., $\|\nabla f_1(\mathbf{w}_{MAML})\|_2 \lesssim \left(\frac{1 - \alpha {\beta_2}}{1 - \alpha L_1}\right)^2 \|\nabla f_2(\mathbf{w}_{MAML})\|_2 + O(\alpha^2)$.
\end{proof}

Now we are ready to prove Theorem \ref{lem:sc}. 

% First, we need to formally state the assumptions on the activation $\sigma$.

% \begin{proposition}[Application of Lemmas D.3, D.10 from \cite{zhong2017recovery}] \label{lem:sc}
% Assume that $\sigma$ satisfies Properties 
% For some $i$, let $\mathbf{\Sigma}_i = \mathbf{I}_d$ and define $s_{i,k}$ as the $k$-th singular value of $\mathbf{W}_{i,\ast}$, $\kappa_i \coloneqq \|\mathbf{W}_{i,\ast}\|_2/s_N$, and $\lambda_i \coloneqq \frac{\Pi_{k=1}^N s_{i,k}}{s_{i,N}^N}$. Then the population loss $f_i$ is strongly convex and smooth in the region $\mathcal{S}_i \coloneqq \{\mathbf{W} : \|\mathbf{W} - \mathbf{W}_{i,\ast}\|_2 \leq c /(\sigma_{i,1}^\gamma \lambda_i \kappa_i^2 N^2)\}$ with parameters $\beta_i \coloneqq \frac{c_1}{\lambda \kappa^2}$ and $L_i \coloneqq c_2 N \sigma_{i,1}^{2\gamma}$, respectively, where $c,c_1,$ and $c_2$ are absolute constants.
% \end{proposition}

\begin{proof}

We first show that  $\beta_i \mathbf{I}_{Nd} \preceq \nabla^2 f_i(\mathbf{W}) \preceq L_i \mathbf{I}_{Nd}$ for all $\mathbf{W} \in \mathcal{S}_i$ for $i \in \{1,2\}$, where $\nabla^2 f_i(\mathbf{W}) \in \mathbb{R}^{Nd\times Nd}$ is the Hessian of the loss of the vectorized $\mathbf{W}$ and each $\beta_i$ and $L_i$ is defined in Theorem \ref{lem:sc}. In other words, we will show that each $f_i$ is $\beta_i$-strongly convex and $L_i$-smooth within $\mathcal{S}_i$.
This will show that any stationary point $\mathbf{W}_{MAML}$ that lies within $\mathcal{S}_1 \cap \mathcal{S}_2$ satisfies the conditions of Lemma \ref{prop:hess}.

For any $i\in\{1,2\}$ and for any $\mathbf{W} \in \mathbb{R}^{d \times N}$ we have by Weyl's Inequality
\begin{align}
    \nabla^2 f_i(\mathbf{W}_{i,\ast}) &- \|\nabla^2 f_i(\mathbf{W}) - \nabla^2 f_i(\mathbf{W}_{i,\ast})\|_2 \mathbf{I}_{Nd}\nonumber\\
    &\preceq \nabla^2 f_i(\mathbf{W}) \preceq \nabla^2 f_1(\mathbf{W}_{i,\ast}) + \|\nabla^2 f_i(\mathbf{W}) - \nabla^2 f_i(\mathbf{W}_{i,\ast})\|_2\mathbf{I}_{Nd} \label{sc1}
\end{align}
Thus, we will control the spectrum of $\nabla^2 f_i(\mathbf{W})$ by controlling the spectrum of $\nabla^2 f_i(\mathbf{W}_{i,\ast})$ and by upper bounding $\|\nabla^2 f_i(\mathbf{W}) - \nabla^2 f_i(\mathbf{W}_{i,\ast})\|_2$. 

To control the spectrum of $\nabla^2 f_i(\mathbf{W}_{i,\ast})$ we use Lemma D.3 from \cite{zhong2017recovery}, which shows that for absolute constants $c_1$ and $c_2$ and each of the possible $\sigma$ functions listed in Theorem \ref{lem:sc},
\begin{align}
(c_1/(\kappa^2 \lambda))\mathbf{I}_{Nd} \preceq \nabla^2 f_1(\mathbf{W}_{i,\ast}) \preceq (c_2 N  s_{i,1}^{2c} )\mathbf{I}_{Nd}. \label{sc2}
\end{align}
Next, we apply Lemma D.10 from \cite{zhong2017recovery}, which likewise applies for all the mentioned $\sigma$, to obtain
\begin{align}
    \|\nabla^2 f_i(\mathbf{W}) - \nabla^2 f_i(\mathbf{W}_{i,\ast})\|_2 \leq c_3 N^2 s_{i,1}^{c} \|\mathbf{W} - \mathbf{W}_{i,\ast}\|_2 \label{sc3}
\end{align}
for a constant $c_3$. Next, for any $\mathbf{W}\in \mathcal{S}_i$, we have $\|\mathbf{W} - \mathbf{W}_{i,\ast}\|_2 = O(1/( s_{i,1}^c \lambda_i \kappa^2_i N^2))$. Therefore, by combining (\ref{sc1}), (\ref{sc2}) and (\ref{sc3}), we obtain that $\beta_i \mathbf{I}_{Nd} \preceq \nabla^2 f_i(\mathbf{W}) \preceq L_i \mathbf{I}_{Nd}$ for all  $\mathbf{W}\in\mathcal{S}_i$.

Finally we apply Lemma \ref{prop:hess} to complete the proof.
\end{proof}

Note that the constant $c$ used in Theorem \ref{lem:sc} is the homogeneity constant for which $\sigma$ satisfies Property 3.1 from \cite{zhong2017recovery}, namely, $0 \leq \sigma'(z) \leq a |z|^c \; \forall z \in \mathbb{R}$.
